# Supplementary material for: Downlink Performance of Superimposed Pilots in Massive MIMO systems
Source: arXiv:1606.04476 source file (2018-03-20)
Supplement: Supplementary file 1 [file appendixDlSinrCalcIterative.tex]

\section{}
\subsection*{Downlink SINR for the Iterative Data-Aided Channel Estimator Based on SP Pilots}
\label{appdx:dlSinrIterative}
This derivation proceeds similar to the derivation in Appendix \ref{appdx:dlSinr}. Assuming that the iterative algorithm is run for $ \numIter_{\sIdxOne} $ iterations at the $ \sIdxOne\rth $ BS, we have 
\begin{align}
\widehat{\dlTxData}_{\vIdxOne,\vIdxTwo}
&= 
\frac{1}{M} 
\lrc{
	\sum\limits_{\sIdxOne}
	\sum\limits_{\sIdxTwo} 
	\lrc{\widehat{\mbf{h}}_{\sIdxOne,\sIdxOne,\sIdxTwo}^{\lrc{\numIter_{\sIdxOne}}}}^H
	\mbf{h}_{\sIdxOne,\vIdxOne,\vIdxTwo}	 
	\dlTxData_{\sIdxOne,\sIdxTwo} 
	+ 
	w_{\vIdxOne,\vIdxTwo} 
}
\nonumber
\\
&=
\mathrm{s}
+
\mathrm{i}
\end{align}
where
\begin{align}
\mathrm{s}
&\triangleq
\channelEstimateIterativeMean{\numIter_{\vIdxOne}}
\dlTxData_{\vIdxOne,\vIdxTwo}
\\
\channelEstimateIterativeMean{\numIter_{\vIdxOne}}
&\triangleq
\frac{1}{M}
\expectation
\lrf{		
		\lrc{\widehat{\mbf{h}}_{\vIdxOne,\vIdxOne,\vIdxTwo}^{\lrc{\numIter_{\vIdxOne}}}}^H
		\mbf{h}_{\vIdxOne,\vIdxOne,\vIdxTwo}
	}
\\
\mathrm{i}
&\triangleq
\lrc{
	\frac{1}{M}
\lrc{\widehat{\mbf{h}}_{\vIdxOne,\vIdxOne,\vIdxTwo}^{\lrc{\numIter_{\vIdxOne}}}}^H
\mbf{h}_{\vIdxOne,\vIdxOne,\vIdxTwo}	
-
\channelEstimateIterativeMean{\numIter_{\vIdxOne}}	
	}
\dlTxData_{\vIdxOne,\vIdxTwo}	
+
\frac{1}{M}
\mathop{
\sum
\sum}_{\lrc{\sIdxOne,\sIdxTwo}\neq\lrc{\vIdxOne,\vIdxTwo}}
\lrc{\widehat{\mbf{h}}_{\sIdxOne,\sIdxOne,\sIdxTwo}^{\lrc{\numIter_{\sIdxOne}}}}^H
\mbf{h}_{\sIdxOne,\vIdxOne,\vIdxTwo}	 
\dlTxData_{\sIdxOne,\sIdxTwo} 		
+ 
\frac{w_{\vIdxOne,\vIdxTwo} }{M} \;.
\end{align}
Then, under the assumptions \ref{S1}-\ref{S3}, $ \channelEstimateIterativeMean{\vIdxOne} $ can be obtained as
\begin{equation}
	\channelEstimateIterativeMean{\vIdxOne} 
	= 
	\beta_{\vIdxOne,\vIdxOne,\vIdxTwo}
	+
	\expectation
	\lrf{
			\lrc{\Delta\mbf{h}^{(\numIter_{\vIdxOne})}_{\vIdxOne,\vIdxOne,\vIdxTwo}}^H
			\mbf{h}_{\vIdxOne,\vIdxOne,\vIdxTwo}
		}
	= 
	\beta_{\vIdxOne,\vIdxOne,\vIdxTwo}\;.
\end{equation}
In addition, under the same assumptions \ref{S1}-\ref{S3}, $ \expectation\lrf{|\mathrm{i}|^2} $ can be obtained as
\begin{align}
	&\expectation\lrf{|\mathrm{i}|^2}
	\!
	=
	\!
		\frac{1}{M^2}
		\expectation
		\lrf{
			\left|\lrc{\widehat{\mbf{h}}_{\vIdxOne,\vIdxOne,\vIdxTwo}^{\lrc{\numIter_{\vIdxOne}}}}^H
			\mbf{h}_{\vIdxOne,\vIdxOne,\vIdxTwo}\right|^2
			\!
		}
	\!
	-
	\!
	\lrc{\channelEstimateIterativeMean{\numIter_{\vIdxOne}}}^2
	+
	\frac{1}{M^2}
	\!
	\mathop{
		\sum
		\sum
		}_{\lrc{\sIdxOne,\sIdxTwo}\neq\lrc{\vIdxOne,\vIdxTwo}}
	\expectation
	\lrf{
	\left|\lrc{\widehat{\mbf{h}}_{\sIdxOne,\sIdxOne,\sIdxTwo}^{\lrc{\numIter_{\sIdxOne}}}}^H
	\mbf{h}_{\sIdxOne,\vIdxOne,\vIdxTwo}\right|^2
	\!
	}
	\!
	+ 
	\!
	\frac{\sigma^2 }{M^2}
	\nonumber\\	
	&=
	-
	\beta_{\vIdxOne,\vIdxOne,\vIdxTwo}^2
	+
	\frac{1}{M^2}
	\sum\limits_{\sIdxOne}
	\sum\limits_{\sIdxTwo}	
	\expectation
	\lrf{
		\left|\lrc{\widehat{\mbf{h}}_{\sIdxOne,\sIdxOne,\sIdxTwo}^{\lrc{\numIter_{\sIdxOne}}}}^H
		\mbf{h}_{\sIdxOne,\vIdxOne,\vIdxTwo}\right|^2
	}
	+ 
	\frac{\sigma^2 }{M^2}
	\nonumber
	\\
	&=
	\frac{1}{M^2}
	\sum\limits_{\sIdxOne}
	\sum\limits_{\sIdxTwo}	
	\expectation
	\lrf{
		\left|\mbf{h}_{\sIdxOne,\sIdxOne,\sIdxTwo}^H
		\mbf{h}_{\sIdxOne,\vIdxOne,\vIdxTwo}\right|^2
	}
	-
	\beta_{\vIdxOne,\vIdxOne,\vIdxTwo}^2
	+
	\frac{2}{M^2}
	\Re
	\lrf{
			\sum\limits_{\sIdxOne}
			\sum\limits_{\sIdxTwo}	
			\expectation
			\lrf{
				\mbf{h}_{\sIdxOne,\sIdxOne,\sIdxTwo}^H
				\mbf{h}_{\sIdxOne,\vIdxOne,\vIdxTwo}	
				\mbf{h}_{\sIdxOne,\vIdxOne,\vIdxTwo}^H
				\lrc{\Delta\mbf{h}_{\sIdxOne,\sIdxOne,\sIdxTwo}^{\lrc{\numIter_{\sIdxOne}}}}				
			}
		}
	\nonumber\\
	&+
	\frac{1}{M^2}
	\sum\limits_{\sIdxOne}
	\sum\limits_{\sIdxTwo}	
	\expectation
	\lrf{
		\left|\lrc{\Delta\mbf{h}_{\sIdxOne,\sIdxOne,\sIdxTwo}^{\lrc{\numIter_{\sIdxOne}}}}^H
		\mbf{h}_{\sIdxOne,\vIdxOne,\vIdxTwo}\right|^2
	}
	+ 
	\frac{\sigma^2 }{M^2}
	\nonumber\\
	&=
	\frac{1}{M}
	\sum\limits_{\sIdxOne}
	\sum\limits_{\sIdxTwo}	
	\beta_{\sIdxOne,\sIdxOne,\sIdxTwo}
	\beta_{\sIdxOne,\vIdxOne,\vIdxTwo}
	+
	\frac{1}{M^2}
	\sum\limits_{\sIdxOne}
	\sum\limits_{\sIdxTwo}	
	\expectation
	\lrf{
		\left|\lrc{\Delta\mbf{h}_{\sIdxOne,\sIdxOne,\sIdxTwo}^{\lrc{\numIter_{\sIdxOne}}}}^H
		\mbf{h}_{\sIdxOne,\vIdxOne,\vIdxTwo}\right|^2
	}
	+ 
	\frac{\sigma^2 }{M^2}
	\;.
	\label{eqn:dlIterativeInterferencePower}
\end{align}
The second term in the above expression, which is given as
\begin{align}
	t_1
	&=
	\frac{1}{M^2} 
	\sum\limits_{\sIdxOne}
	\sum\limits_{\sIdxTwo}
	\expectation
	\lrf{
		|\lrc{\Delta\mbf{h}_{\sIdxOne,\sIdxOne,\sIdxTwo}^{\numIter_{\sIdxOne}}}^H
		\mbf{h}_{\sIdxOne,\vIdxOne,\vIdxTwo}|^2
	}
	\label{eqn:b4InterimIterative}
\end{align}
can be simplified as follows.
From \eqref{eqn:iterativeChannelEstimate}, the error in the channel estimate $ \widehat{\mbf{h}}_{\sIdxOne,\sIdxOne,\sIdxTwo}^{\lrc{\numIter_{\sIdxOne}}} $ can be written as
\begin{align}
	&\Delta\mbf{h}_{\sIdxOne,\sIdxOne,\sIdxTwo}^{(\numIter_{\sIdxOne})} 
	= 
	-\frac{\rhoD{}{}}{\ulDuration\rhoP{}{}}
	\Bigg(	
	\mathop{
	\sum
	\sum
	}_{\substack{\ordering\lrc{\sIdxThree,\sIdxFour}<\ordering\lrc{\sIdxOne,\sIdxTwo}\\\lrc{\sIdxThree,\sIdxFour}\in\mathcal{U}_{\sIdxOne,\sIdxOne,\sIdxTwo}^{(\numIter_{\sIdxOne})}}}
	\left\{
	\mbf{h}_{\sIdxOne,\sIdxThree,\sIdxFour}
	\lrc{\Delta\mbf{x}_{\sIdxThree,\sIdxFour}^{(\numIter_{\sIdxOne})} }^T
	+ 
	\Delta\mbf{h}_{\sIdxOne,\sIdxThree,\sIdxFour}^{(\numIter_{\sIdxOne})}
	\mbf{x}_{\sIdxThree,\sIdxFour}^T -
	\Delta\mbf{h}_{\sIdxOne,\sIdxThree,\sIdxFour}^{(\numIter_{\sIdxOne})}
	\!\!
	\lrc{\Delta\mbf{x}_{\sIdxThree,\sIdxFour}^{(\numIter_{\sIdxOne})}}^T 
	\right\}\!
	+
	\mbf{W}_{\sIdxOne}
	\nonumber\\
	&
	\!
	+
	\!\!\!
	\mathop{
		\sum
		\sum}_{\lrc{\sIdxThree,\sIdxFour}\notin\mathcal{U}_{\sIdxOne,\sIdxOne,\sIdxTwo}}
	\!\!
	\mbf{h}_{\sIdxOne,\sIdxThree,\sIdxFour}
	\mbf{x}_{\sIdxThree,\sIdxFour}^T
	+
	\!\!\!\!\!
	\mathop{
	\sum
	\sum
	}_{\substack{\ordering\lrc{\sIdxThree,\sIdxFour}\geq\ordering\lrc{\sIdxOne,\sIdxTwo}\\\lrc{\sIdxThree,\sIdxFour}\in\mathcal{U}_{\sIdxOne,\sIdxOne,\sIdxTwo}^{(\numIter_{\sIdxOne})}}}
	\!\!\!\!
	\left\{		
	\mbf{h}_{\sIdxOne,\sIdxThree,\sIdxFour}
	\!
	\lrc{\!\Delta\mbf{x}_{\sIdxThree,\sIdxFour}^{(\numIter_{\sIdxOne}-1)}\!}^T\!
	\!
	+
	\!
	\Delta\mbf{h}_{\sIdxOne,\sIdxThree,\sIdxFour}^{(\numIter_{\sIdxOne}-1)}
	\mbf{x}_{\sIdxThree,\sIdxFour}^T	
	- 
	\Delta\mbf{h}_{\sIdxOne,\sIdxThree,\sIdxFour}^{(\numIter_{\sIdxOne}-1)}
	\!\!
	\lrc{\Delta\mbf{x}_{\sIdxThree,\sIdxFour}^{(\numIter_{\sIdxOne}-1)}}^T
	\!
	\right\}
	\!\!
	\Bigg)
	\mbf{p}_{\sIdxOne,\sIdxTwo}^*
	\;.
	\label{eqn:deltaHdefn}
\end{align}
Then, we can define the term in the summation in \eqref{eqn:b4InterimIterative} as
\begin{align}
	\psi_{\sIdxOne,\sIdxTwo,\vIdxOne,\vIdxTwo}^{(\numIter_{\sIdxOne})}
	&\triangleq
	\expectation
	\lrf{
		\lrc{\Delta\mbf{h}_{\sIdxOne,\sIdxOne,\sIdxTwo}^{\lrc{\numIter_{\sIdxOne}}}}^H
		\mbf{h}_{\sIdxOne,\vIdxOne,\vIdxTwo}
		\mbf{h}_{\sIdxOne,\vIdxOne,\vIdxTwo}^H
		\Delta\mbf{h}_{\sIdxOne,\sIdxOne,\sIdxTwo}^{\lrc{\numIter_{\sIdxOne}}}
	}\;.
	\label{eqn:psiDefn}
\end{align}
Using \eqref{eqn:deltaHdefn} and the assumptions \ref{S1}-\ref{S3} in \eqref{eqn:psiDefn}, we can simplify \eqref{eqn:psiDefn} to obtain \eqref{eqn:psiEqn}. Substituting \eqref{eqn:psiDefn} and \eqref{eqn:b4InterimIterative} into \eqref{eqn:dlIterativeInterferencePower}, the interference power in the DL when the iterative data-aided method is used for channel estimation can be obtained as
\begin{align}
	\expectation\lrf{|\mathrm{i}|^2}
	&=
	\frac{1}{M}
	\sum\limits_{\sIdxOne}
	\sum\limits_{\sIdxTwo}	
	\beta_{\sIdxOne,\sIdxOne,\sIdxTwo}
	\beta_{\sIdxOne,\vIdxOne,\vIdxTwo}
	+
	\frac{1}{M^2} 
	\sum\limits_{\sIdxOne}
	\sum\limits_{\sIdxTwo}
	\psi_{\sIdxOne,\sIdxTwo,\vIdxOne,\vIdxTwo}^{(\numIter_{\sIdxOne})}
	+
	\frac{\sigma^2}{M^2}\;.
\end{align} 
The DL SINR with $ \numIter_{\sIdxOne} $ can finally be obtained as
\begin{align}
	\sinrDlIterative_{\vIdxOne,\vIdxTwo}
	= 
	\frac{\beta_{\vIdxOne,\vIdxOne,\vIdxTwo}^2}{\expectation\lrf{|\mathrm{i}|^2}}\;.
\end{align}
This completes the derivation of \eqref{eqn:dlSinrIterative}.
